# Supplementary material for: EasyST: A Simple Framework for Spatio-Temporal Prediction
Source: arXiv:2409.06748 source file (2024-09-10)
Supplement: Supplementary file 1 [file appendix.tex]

\section{Appendix}
\label{tab:appendix}
